# Supplementary material for: Energy criterion for the spectral stability of discrete breathers
Source: arXiv:1604.06956 ancillary file (2016-08-24)
Supplement: Supplementary file 1 [file SupplementaryMaterial.pdf]

# Supplement:

## An energy criterion for the spectral stability of discrete breathers

Panayotis G. Kevrekidis

*Department of Mathematics and Statistics, University of Massachusetts, Amherst, MA 01003-9305, USA*

Jesús Cuevas-Maraver

*Grupo de Física No Lineal, Departamento de Física Aplicada I,*

*Universidad de Sevilla. Escuela Politécnica Superior, C/ Virgen de África, 7, 41011-Sevilla, Spain*

*Instituto de Matemáticas de la Universidad de Sevilla (IMUS). Edificio Celestino Mutis. Avda. Reina Mercedes s/n, 41012-Sevilla, Spain*

Dmitry E. Pelinovsky

*Department of Mathematics, McMaster University, Hamilton, Ontario, Canada, L8S 4K1*

*Department of Applied Mathematics, Nizhny Novgorod State Technical University, 24 Minin Street, Nizhny Novgorod, Russia, 603 950*

**Derivation of the expansion (7).** We consider the linear eigenvalue problem for the 1D KG chain:

$$\omega^2 W_n''(\tau) + 2\lambda\omega W_n'(\tau) + \lambda^2 W_n(\tau) + V''(U_n(\tau))W_n(\tau) = C(\Delta W)_n(\tau), \quad (1)$$

where  $U(\tau) \in H_{\text{per}}^2((0, 2\pi); \ell^2(\mathbb{Z}))$  is a time-periodic breather localized over the lattice with the frequency  $\omega$ ,  $\lambda \in \mathbb{C}$  is a spectral parameter and  $W(\tau) \in H_{\text{per}}^2((0, 2\pi); \ell^2(\mathbb{Z}))$  is an eigenvector of the spectral problem.

We recall that  $W_n(\tau) = U_n'(\tau)$  is an eigenvector of (1) for  $\lambda = 0$  generated by the time translation symmetry (associated with the energy conservation). In addition,  $\tilde{W}_n(\tau) = \partial_\omega U_n(\tau)$  satisfies the derivative of (1) in  $\lambda$  for  $\lambda = 0$ , that is, it represents the generalized eigenvector of (1) for  $\lambda = 0$  generated by a shift of frequency. Indeed, the breather equation

$$\omega^2 U_n''(\tau) + V'(U_n(\tau)) = C(\Delta U)_n(\tau) \quad (2)$$

implies that

$$(L\partial_\omega U)_n(\tau) = 2\omega U_n''(\tau), \quad (3)$$

where

$$(LW)_n(\tau) = C(\Delta W)_n(\tau) - V''(U_n(\tau))W_n(\tau) - \omega^2 W_n''(\tau) \quad (4)$$

is the linearized operator for the spectral problem (1) acting on a sequence of functions in  $H_{\text{per}}^2((0, 2\pi); \ell^2(\mathbb{Z}))$  with the range in  $L^2((0, 2\pi); \ell^2(\mathbb{Z}))$ . We assume the following:

- The spectral bands of (1) in the linearization of the zero equilibrium  $U_n(\tau) \equiv 0$  are bounded away from  $\lambda = 0$ ,
- The kernel of  $L$  is exactly one-dimensional with the eigenvector  $W_n(\tau) = U_n'(\tau)$ .
- The dependence of breathers  $U(\tau)$  and its energy  $H$  on the frequency  $\omega$  is smooth and has a critical point  $\omega_0$ , where  $H'(\omega_0) = 0$ .

At  $\omega = \omega_0$ , we are looking for a formal expansion of solutions to the linear eigenvalue problem (1) in powers of  $\lambda$ :

$$W_n(\tau) = U_n'(\tau) + \lambda\partial_\omega U_n(\tau) + \lambda^2 Y_n(\tau) + \lambda^3 Z_n(\tau) + \lambda^4 P_n(\tau) + \mathcal{O}(\lambda^5). \quad (5)$$

Substituting (5) to (1), we obtain a chain of linear inhomogeneous equations

$$(LY)_n(\tau) = 2\omega\partial_\omega U_n'(\tau) + U_n'(\tau), \quad (6)$$

$$(LZ)_n(\tau) = 2\omega Y_n'(\tau) + \partial_\omega U_n(\tau), \quad (7)$$

$$(LP)_n(\tau) = 2\omega Z_n'(\tau) + Y_n(\tau). \quad (8)$$

Projecting (6) to the homogeneous solution  $W_n = U'_n(x)$  and integrating by parts yields the Fredholm solvability condition in the form

$$\begin{aligned} 0 &= \int_0^{2\pi} \sum_{n \in \mathbb{Z}} U'_n(\tau) [2\omega \partial_\omega U'_n(\tau) + U'_n(\tau)] d\tau \\ &= \omega^{-1} \int_0^{2\pi} \sum_{n \in \mathbb{Z}} [\omega^2 U'_n(\tau) \partial_\omega U'_n(\tau) - \omega^2 U''_n(\tau) \partial_\omega U_n(\tau) + \omega [U'_n(\tau)]^2] d\tau = TH'(\omega), \end{aligned}$$

where we have introduced the time-independent breather energy

$$H(\omega) = \sum_{n \in \mathbb{Z}} \frac{1}{2} \omega^2 [U'_n(\tau)]^2 + V(U_n(\tau)) + \frac{1}{2} C (U_{n+1}(\tau) - U_n(\tau))^2 \quad (9)$$

and used the breather equation (2) for the derivative  $H'(\omega)$ . The solvability condition is satisfied if  $\omega = \omega_0$  is a critical point of the breather energy  $H(\omega)$ . In this case, there is a solution  $\{Y_n(\tau)\}_{n \in \mathbb{Z}} \in H_{\text{per}}^2((0, 2\pi); \ell^2(\mathbb{Z}))$  to the linear equation (6), which can be made unique if it is orthogonal to the eigenvector  $W_n(\tau) = U'_n(\tau)$ . Moreover, if  $U_n(\tau)$  is even in  $\tau$ , then  $Y_n(\tau)$  is odd in  $\tau$ .

The Fredholm solvability condition is satisfied for the linear equation (7) because the parity of  $Y'_n(\tau)$  and  $\partial_\omega U_n(\tau)$  is opposite to the parity of  $U'_n(\tau)$ . Therefore, there exists a unique even solution  $\{Z_n(\tau)\}_{n \in \mathbb{Z}} \in H_{\text{per}}^2((0, 2\pi); \ell^2(\mathbb{Z}))$  to the linear equation (7), which is thus orthogonal to the odd function  $W_n(\tau) = U'_n(\tau)$ .

Finally, the linear inhomogeneous equation (8) does not have a solution in  $H_{\text{per}}^2((0, 2\pi); \ell^2(\mathbb{Z}))$  if the eigenvalue  $\lambda = 0$  is exactly quadruple. The quantity  $M$  appearing in the expansion (8) of the main text is obtained by projecting the linear equation (8) to the homogeneous solution  $W_n = U'_n(x)$ , namely,

$$\begin{aligned} M &= \int_0^{2\pi} \sum_{n \in \mathbb{Z}} U'_n(\tau) [2\omega Z'_n(\tau) + Y_n(\tau)] d\tau \\ &= \int_0^{2\pi} \sum_{n \in \mathbb{Z}} [U'_n(\tau) Y_n(\tau) - 2\omega U''_n(\tau) Z_n(\tau)] d\tau \\ &= \int_0^{2\pi} \sum_{n \in \mathbb{Z}} ([U'_n(\tau) + 2\omega \partial_\omega U'_n(\tau)] Y_n(\tau) - [\partial_\omega U_n(\tau)]^2) d\tau, \end{aligned}$$

where we have used the linear inhomogeneous equations (3) and (7), smoothness and decay of  $U_n$ ,  $Y_n$  and  $Z_n$ , as well as the self-adjoint properties of  $L$ .

We need to compute the sign of  $M$  in order to detect the regions where instability of breathers arises. Combining projections to the linear equations (6) and (8), we obtain the expansion

$$\lambda^2 TH'(\omega) + \lambda^4 M + \mathcal{O}(\lambda^6) = 0. \quad (10)$$

Expansion (10) shows how the zero eigenvalue of quadruple multiplicity splits if  $\omega$  is close to but not equal to  $\omega_0$ , the critical point of  $H$ . Justification of the expansion (10) for small  $|\omega - \omega_0|$  can be constructed similarly to the perturbation theory used in [1]. If  $M > 0$ , the expansion (10) shows that  $\lambda^2 < 0$  if  $H'(\omega) > 0$  and  $\lambda^2 > 0$  if  $H'(\omega) < 0$ , whereas if  $M < 0$ , then  $\lambda^2 < 0$  if  $H'(\omega) < 0$  and  $\lambda^2 > 0$  if  $H'(\omega) > 0$ , where  $\lambda^2$  corresponds to the pair of either purely imaginary or real eigenvalues that split from the double zero eigenvalue if  $\omega \neq \omega_0$  and  $H'(\omega) \neq 0$ .

It does not look feasible to compute the sign of  $M$  in a general case. However, working with small-amplitude breathers and asymptotic multi-scale expansions, we can approximate KG breathers with the discrete nonlinear Schrödinger (dNLS) equation [2] and thus obtain a definite conclusion on the sign of  $M$  depending on whether the nonlinear potential  $V$  is hard or soft. Similar expansions can be derived for the FPU lattice in strain variables, where the existence of breathers was studied earlier with the dNLS equation based on the central manifold theory near optical frequencies [3, 4]. In both cases, we prove next that  $M > 0$  for hard potentials and  $M < 0$  for soft potentials. Therefore, the fundamental breathers with increasing frequency-energy dependence are stable in hard potentials and unstable in soft potentials and vice versa for the decreasing frequency-energy dependence.

**Small-amplitude limit of KG breathers.** We consider the on-site potential in the form  $V'(u) = u \pm \epsilon u^{1+2p}$ , where  $\epsilon$  is a small positive parameter,  $p$  is a positive integer, and the plus/minus sign corresponds to the hard/soft potential. Using the asymptotic approximation of small-amplitude breathers [2],

$$U_n(\tau) = A_n e^{i\tau} + \bar{A}_n e^{-i\tau} + \mathcal{O}(\epsilon), \quad (11)$$

we obtain from (2) the stationary dNLS equation for the amplitude sequence  $\{A_n\}_{n \in \mathbb{Z}} \in \ell^2(\mathbb{Z})$ :

$$\epsilon^{-1} C(\Delta A)_n = \epsilon^{-1} (1 - \omega^2) A_n \pm \gamma |A_n|^{2p} A_n, \quad n \in \mathbb{Z}, \quad (12)$$

where  $\gamma = (2p+1)!/(p!(p+1)!)$  is a numerical constant. It is well-known [5] that a homoclinic orbit to the stationary dNLS equation (12) exists for hard potentials (upper sign) if  $\omega^2 > 1 + 4C$  and for soft potentials (lower sign) if  $\omega^2 < 1$ . Moreover, as  $\epsilon \rightarrow 0$ , the homoclinic orbit can be approximated by the NLS sech soliton [6] if  $\omega^2 = 1 + 4C + \epsilon\Omega$  in the former case and  $\omega^2 = 1 - \epsilon\Omega$  in the latter case, where  $\Omega$  is a positive  $\epsilon$ -independent parameter. Without loss of generality,  $\{A_n\}_{n \in \mathbb{Z}} \in \ell^2(\mathbb{Z})$  can be considered to be real, moreover, the sequence is strictly positive for soft potentials and sign-alternating for hard potentials [5].

Using (9) and (11), we have  $H(\omega) = 2\omega^2 P(\Omega) + \mathcal{O}(\epsilon)$  with the power (also known as mass or charge)  $P(\omega) = \|A\|_{\ell^2}^2$ , therefore,

$$H'(\omega) = \pm 4\omega^3 \epsilon^{-1} P'(\Omega) + \mathcal{O}(1), \quad (13)$$

where the sign of  $P'(\Omega)$  determines the stability of NLS solitons according to the Vakhitov–Kolokolov (VK) slope condition [7]. Thus, in the small-amplitude limit of KG breathers, the change of monotonicity of  $P'(\Omega)$  in the dNLS equation is tantamount to the change of monotonicity of the energy  $H'(\omega)$  in the KG lattice.

Using the approximation (11), we find the leading-order contribution to the linear inhomogeneous equation (6) in the form

$$Y_n(\tau) = i\epsilon^{-2} [B_n e^{i\tau} - \bar{B}_n e^{-i\tau}] + \mathcal{O}(\epsilon^{-1}), \quad (14)$$

where the sequence  $\{B_n\}_{n \in \mathbb{Z}}$  satisfies the linear inhomogeneous equation

$$(L_- B)_n = \pm 4\omega^2 \partial_\Omega A_n, \quad (15)$$

where

$$(L_- B)_n = \epsilon^{-1} C(\Delta B)_n - \epsilon^{-1} (1 - \omega^2) B_n \mp \gamma |A_n|^{2p} B_n \quad (16)$$

is the linearized operator for the stationary dNLS equation (12) associated with the imaginary part of the perturbation to the stationary mode  $\{A_n\}_{n \in \mathbb{Z}}$ .  $L_-$  is a bounded discrete Schrödinger operator defined on  $\ell^2(\mathbb{Z})$  for every  $\epsilon > 0$ . Since  $(L_- A)_n = 0$  and  $\{A_n\}_{n \in \mathbb{Z}}$  is real and strictly positive for soft potentials or sign-alternating for hard potentials, the spectrum of  $L_-$  is sign definite. It is easy to show that  $L_-$  is positive for hard potentials and negative for soft potentials. Furthermore, for every sufficiently small  $\epsilon$ , there is an  $\epsilon$ -independent constant  $C$  such that

$$\pm \langle L_- B, B \rangle_{\ell^2} \geq C \|B\|_{\ell^2}^2 \quad (17)$$

for every  $B$  orthogonal to  $A$  [6].

Since  $(L_- A)_n = 0$ , there exists a solution to the linear inhomogeneous equation (15) if and only if  $P'(\Omega) = 0$ . This Fredholm solvability condition represents the reduced energy condition that comes from the expansion (13). Moreover, a solution  $\{B_n\}_{n \in \mathbb{Z}}$  is unique if it is defined to be orthogonal to the homogeneous solution  $\{A_n\}_{n \in \mathbb{Z}}$ . Substituting (11) and (14) into the expression for  $M$  in (10), we obtain

$$M = 4\pi\epsilon^{-3} \langle L_- B, B \rangle_{\ell^2} + \mathcal{O}(\epsilon^{-2}). \quad (18)$$

Thanks to the bounds (17), the leading-order contribution for  $M$  in (18) occurs at the order  $\mathcal{O}(\epsilon^{-3})$  and it is sign-definite. Therefore, we have  $M > 0$  for hard potentials and  $M < 0$  for soft potentials, if  $\epsilon$  is sufficiently small. As follows from the expansion (10), the small-amplitude breathers of the KG lattice are stable if  $H'(\omega) > 0$  and unstable if  $H'(\omega) < 0$  for hard potentials, and vice versa for soft potentials.

**Breathers in FPU lattices.** Discrete breathers of the FPU lattice have to be reformulated in the variable  $r_n = u_{n+1} - u_n$  in the sequence space  $\ell^2(\mathbb{Z})$ , since  $\{u_n\}_{n \in \mathbb{Z}}$  is no longer decaying at infinity. Therefore, we can modify all the expressions starting with the FPU equation

$$\ddot{r}_n = W'(r_{n+1}) - 2W'(r_n) + W'(r_{n-1}), \quad n \in \mathbb{Z}. \quad (19)$$

Implementing the change in notations  $u_n \rightarrow r_n$ , the rest of our analysis is repeated verbatimly and results in the condition  $H'(\omega) = 0$ , where the breather energy is now given by

$$H(\omega) = \sum_{n \in \mathbb{Z}} \frac{1}{2} \omega^2 [U'_n(\tau)]^2 + W(R_n(\tau)), \quad R_n(\tau) := U_{n+1}(\tau) - U_n(\tau). \quad (20)$$

We can also obtain the same expansion (10) with the same expression for quantity  $M$ . The necessity to work with the strain variable can be understood by looking at the generalized eigenvector  $\tilde{W}_n(\tau) = \partial_\omega U_n(\tau)$  satisfying the linear inhomogeneous equation (3). This sequence does not decay to zero at infinity in  $n$ , whereas it does decay to zero and is well defined in  $H_{\text{per}}^2((0, 2\pi); \ell^2(\mathbb{Z}))$  in the strain variable  $\partial_\omega R_n(\tau)$ .

Next, we show that  $M > 0$  in the small-amplitude limit of FPU breathers in monoatomic chains. In monoatomic chains, the small-amplitude breathers only exist in hard inter-site potential  $W$  [3]. Let the inter-site potential be taken in the form  $W'(u) = Cu + \epsilon u^{1+2p}$ , where  $\epsilon$  is a small positive parameter and  $p$  is a positive integer. Using the asymptotic approximation of small-amplitude breathers [3],

$$R_n(\tau) = A_n e^{i\tau} + \bar{A}_n e^{-i\tau} - \epsilon (A_n e^{i\tau} + \bar{A}_n e^{-i\tau})^{1+2p} + \mathcal{O}(\epsilon^2), \quad (21)$$

we obtain the stationary dNLS equation for the amplitude sequence

$$\epsilon^{-1} C(\Delta A)_n = 4\gamma |A_n|^{2p} A_n - \epsilon^{-1} \omega^2 A_n, \quad n \in \mathbb{Z}, \quad (22)$$

where  $\gamma = (2p+1)!/(p!(p+1)!)$  is the same numerical constant. A homoclinic orbit to the stationary dNLS equation (22) exists now for  $\omega^2 > 4C$  [5] and has similar properties with that in (12). In particular, setting  $\omega^2 = 4C + \epsilon\Omega$  with a positive  $\epsilon$ -independent parameter  $\Omega$ , one can proceed similarly to the analysis of small-amplitude limit of KG breathers and obtain  $M > 0$  for hard inter-site potentials. Thus, the small-amplitude breathers of the monotonic FPU lattice with hard inter-site potential  $W$  are stable if  $H'(\omega) > 0$  and unstable if  $H'(\omega) < 0$ .

**Energy criterion in the AC limit of KG lattices.** The stability threshold  $H'(\omega) = 0$  cannot be achieved near the AC limit  $C = 0$  for the KG lattice. Indeed, if  $T(E)$  is the energy-period dependence of an individual oscillator satisfying  $\ddot{\varphi} + V'(\varphi) = 0$  and its first-order invariant is  $E = \frac{1}{2}\dot{\varphi}^2 + V(\varphi)$ , then

$$H'(\omega) \rightarrow -\frac{T}{\omega T'(E)}$$

in the AC limit. Since  $T'(E)$  cannot be infinite for an individual oscillator satisfying the second-order differential equation,  $H'(\omega)$  is sign-definite. Moreover,  $H'(\omega) > 0$  for hard potentials with  $T'(E) < 0$  and  $H'(\omega) < 0$  for soft potentials with  $T'(E) > 0$ . The individual oscillator is always stable, therefore, the fundamental breather of the KG lattice in the AC limit is stable with  $H'(\omega) > 0$  for hard potentials and  $H'(\omega) < 0$  for soft potentials.

**Description of the numerical methods used for calculating discrete breathers.** Let us recall that a 1D nonlinear lattice equation can be expressed as:

$$\ddot{u}_n + V'(u_n) = W'(u_{n+1} - u_n) - W'(u_n - u_{n-1}), \quad (23)$$

whereas the 2D generalization is given by

$$\ddot{u}_{n,m} + V'(u_{n,m}) = W'(u_{n+1,m} - u_{n,m}) - W'(u_{n,m} - u_{n-1,m}) + W'(u_{n,m+1} - u_{n,m}) - W'(u_{n,m} - u_{n,m-1}). \quad (24)$$

We will explain below the numerical methods used for calculating discrete breather solutions and analyzing their stability in the 1D case, being the generalization to the 2D case straightforward.

In order to calculate periodic orbits in the system (23), we make use of the Fourier series approximations and a path-following (Newton-Raphson) method for continuations of solutions in frequency. Applications of the Fourier methods is enabled by the fact that the breather solutions are  $T$ -periodic; for a detailed explanation of these methods, the reader is referred to Refs. [8, 9]. The method has the advantage, among others, of providing an explicit, analytical form of the Jacobian. Thus, a periodic orbit solution can be expressed in terms of a truncated Fourier series expansion:

$$u_n(t) = \sum_{k=-k_m}^{k_m} z_{k,n} \exp(ik\omega t) \quad (25)$$

with  $k_m$  being the maximal index in the Galerkin truncation. Substituting (25) into (23) yields a set of  $N \times (2k_m + 1)$  coupled algebraic equations:

$$-\omega^2 k^2 z_{k,n} + \mathcal{F}_k[V'(u_n)] - \mathcal{F}_k[W'(u_{n+1} - u_n)] + \mathcal{F}_k[W'(u_n - u_{n-1})] = 0, \quad (26)$$

where  $\mathcal{F}_k$  denotes the Discrete Fourier Transform at  $k$ . As  $u_n(t)$  in (25) must be a real, it implies that  $z_{-k,n} = z_{k,n}^*$ .

Notice that in the case of Klein–Gordon lattices,  $W'(u) = Cu$ , breathers are found by making use of the anti-continuous limit concept [10]. That is, a breather at the limit  $C = 0$  is composed by one (or more) excited oscillator(s) with the remaining ones at rest. Then, this solution is continued by varying the coupling constant  $C$  up to the prescribed value. In the case of FPU lattices, the anti-continuous limit is attained by supposing a diatomic lattice with the masses  $M_n$  so that  $M_n = 1$  for even sites and  $M_n = 1/\epsilon^2$  for odd sites; then, at  $\epsilon = 0$  the odd site masses are infinite and the oscillators decouple.

In order to study the spectral stability of periodic orbits, we introduce a small perturbation  $\{\xi_n(t)\}$  to a given breather solution  $\{u_n(t)\}$  of the system (23). Then, the linearized equations satisfied to first order in  $\xi_n$  read:

$$\ddot{\xi}_n + V''(u_n)\xi_n - W''(u_{n+1} - u_n)(\xi_{n+1} - \xi_n) + W''(u_n - u_{n-1})(\xi_n - \xi_{n-1}) = 0. \quad (27)$$

Floquet analysis of the linearized equations (27) can be performed if  $\{u_n(t)\}$  is the  $T$ -periodic solution, so that the map  $\{u_n(0), \dot{u}_n(0)\} \rightarrow \{u_n(T), \dot{u}_n(T)\}$  has a fixed point. Then, the stability properties of breathers are defined by the spectrum of the Floquet operator  $\mathcal{M}$  given by

$$\begin{pmatrix} \{\xi_n(T)\} \\ \{\dot{\xi}_n(T)\} \end{pmatrix} = \mathcal{M} \begin{pmatrix} \{\xi_n(0)\} \\ \{\dot{\xi}_n(0)\} \end{pmatrix}. \quad (28)$$

The  $2N \times 2N$  eigenvalues  $\mu = \exp(i\theta)$  of  $\mathcal{M}$  are dubbed the *Floquet multipliers* with  $\theta$  being *Floquet exponents*.

- 
- [1] D.E. Pelinovsky and A. Sakovich, *Nonlinearity* **25**:3423–3451 (2012).
  - [2] D. Pelinovsky, T. Penati, and S. Paleari, arXiv:1509.06389.
  - [3] G. James, *J. Nonlin. Sci.* **13** (2003), 27–63.
  - [4] G. James, B. Sánchez-Rey, and J. Cuevas, *Rev. Math. Phys.* **21** (2009), 1–59.
  - [5] W.-X. Qin and X. Xiao, *Nonlinearity* **20** (2007), 2305–2317.
  - [6] D.E. Pelinovsky and G. Schneider, arXiv:1603.05463.
  - [7] N.G. Vakhitov and A.A. Kolokolov, *Radiophys. Quantum Electron.* **16** 783 (1973).
  - [8] J. Cuevas, J.F.R. Archilla, and F.R. Romero, *J. Phys. A: Math. Theor.* **44**, 035102 (2011).
  - [9] J.F.R. Archilla, R.S. MacKay, and J.L. Marín, *Physica D* **134**, 406 (1999).
  - [10] R.S. MacKay and S. Aubry, *Nonlinearity* **7**, 1623 (1994).
